# Supplementary material for: Towards Urban General Intelligence: A Review and Outlook of Urban Foundation Models
Source: arXiv:2402.01749 source file (2026-03-22)
Supplement: Supplementary file 2 [file v4_appendix.tex]

\appendix
% [Summary of Existing Works]

% \small
% \tiny
% \footnotesize
\scriptsize
% \rowcolors{3}{gray!25}{white}
% \begin{tabularx}{\textwidth}{ 
%     >{\centering\arraybackslash}X
%     >{\centering\arraybackslash}X
%     >{\centering\arraybackslash}X
%     >{\centering\arraybackslash}X
%     >{\centering\arraybackslash}X
%     >{\centering\arraybackslash}X
%     >{\centering\arraybackslash}X
%     }
\begin{tabularx}{\textwidth}{ YYYYYYY }
    \caption{Summary of existing works.} \label{table:summary} \\
    \toprule
    % \rowcolor{gray!50}
    \textbf{Study} & \textbf{Data Type} & \textbf{Pre-training} & \textbf{Adaptation} & \textbf{Cross-modal transfer} & \textbf{Cross-domain transfer} & \textbf{Application} \\
    \midrule
    \endfirsthead

    \multicolumn{7}{c}{{\bfseries Table \thetable\ Summary of existing works (continued).}} \\
    \toprule
    % \rowcolor{gray!50}
    \textbf{Study} & \textbf{Data Type} & \textbf{Pre-training} & \textbf{Adaptation} & \textbf{Cross-modal transfer} & \textbf{Cross-domain transfer} & \textbf{Application} \\
    \midrule
    \endhead

    \midrule
    \multicolumn{7}{r}{{Continued on next page}} \\ 
    \endfoot

    \bottomrule
    \endlastfoot

    \multicolumn{7}{c}{\textbf{Language-based Models}} \\
    \hline
    \rowcolor{gray!25} ERNIE-GeoL~\cite{huang2022ernie} & POI corpus, user behavior logs & Generative & Model fine-tuning & - & - & Map services \\
    \cline{1-7}
    MGeo~\cite{ding2023mgeo} & POI corpus & Generative, contrastive & Model fine-tuning & - & - & Query-POI matching \\
    \cline{1-7}
    \rowcolor{gray!25} Ji et al.~\cite{ji2023evaluating} & Geo-text, user instructions & - & Prompt engineering & - & General to geospatial & Geographic information systems \\
    \cline{1-7}
    Bhandari et al.~\cite{bhandari2023large} & Geo-text, user instructions & - & Prompt engineering & - & General to geospatial & Geographic information systems \\
    \cline{1-7}
    \rowcolor{gray!25} GPT4GEO~\cite{roberts2023gpt4geo} & Geo-text, user instructions & - & Prompt engineering & - & General to geospatial & Geographic information systems \\
    \cline{1-7}
    Mooney et al.~\cite{mooney2023towards} & Geo-text, user instructions & - & Prompt engineering & - & General to geospatial & Geographic information systems \\
    \cline{1-7}
    \rowcolor{gray!25} Mai et al.~\cite{mai2023opportunities} & Geo-text, user instructions & - & Prompt engineering & - & General to geospatial & Geographic information systems \\
    \cline{1-7}
    Fu et al.~\cite{fu2023towards} & Documents, geo-text, user instructions & - & Prompt engineering & - & General to urban science & Urban science \\
    \cline{1-7}
    \rowcolor{gray!25} Aghzal et al.~\cite{aghzal2023can} & Geo-text, user instructions & - & Prompt engineering & - & General to path planning & Path planning \\
    \cline{1-7}
    GeoLLM~\cite{manvi2023geollm} & POI corpus & - & Prompt engineering & - & General to geospatial & Geospatial prediction \\
    \cline{1-7}
    \rowcolor{gray!25} Zheng et al.~\cite{zheng2023chatgpt} & Traffic documents, user instructions & - & Prompt engineering & - & General to transportation & Intelligent transportation \\
    \cline{1-7}
    SpaBERT~\cite{li2022spabert} & Geo-text & - & Model fine-tuning & - & General to geospatial & Geographic language understanding \\
    \cline{1-7}
    \rowcolor{gray!25} GeoLM~\cite{li2023geolm} & Geo-text & - & Model fine-tuning & - & General to geospatial & Geographic language understanding \\
    \cline{1-7}
    QUERT~\cite{xie2023quert} & User behavior logs & - & Model fine-tuning & - & General to travel search & Travel query understanding \\
    \cline{1-7}
    \rowcolor{gray!25} GEDR~\cite{mei2023improving} & POI corpus, user behavior logs & - & Model fine-tuning & - & General to POI search & Query-POI matching \\
    \cline{1-7}
    Wang et al.~\cite{wang2023optimizing} & LLM-generated instructions & - & Model fine-tuning & - & General to urban renewal & Urban renewal \\
    \cline{1-7}
    \rowcolor{gray!25} K2~\cite{deng2023learning} & Geo-text, geoscience instructions & - & Model fine-tuning & - & General to geoscience & Geoscience tasks \\
    \midrule[0.5pt]
    
    % Vision-based Models
    \multicolumn{7}{c}{\textbf{Vision-based Models}} \\
    \cline{1-7}
    \rowcolor{gray!25} Urban2vec~\cite{wang2020urban2vec} & Street-view images & Contrastive & Model fine-tuning & - & - & Demographic prediction, socioeconomic prediction \\
    \cline{1-7}
    Li et al.~\cite{li2022predicting} & Street-view images & Contrastive & Model fine-tuning & - & - & Socioeconomic prediction \\
    \cline{1-7}
    \rowcolor{gray!25} KnowCL~\cite{liu2023knowledge} & Street-view images & Contrastive & Model fine-tuning & - & - & Socioeconomic prediction \\
    \cline{1-7}
    Wang et al.~\cite{wang2022advancing} & Remote sensing images & Generative & Model fine-tuning & - & - & Remote sensing image analysis \\
    \cline{1-7}
    \rowcolor{gray!25} ScaleMAE~\cite{reed2023scale} & Remote sensing images & Generative & Model fine-tuning & - & - & Remote sensing image analysis \\
    \cline{1-7}
    Cha et al.~\cite{cha2023billion} & Remote sensing images & Generative & Model fine-tuning & - & - & Remote sensing image analysis \\
    \cline{1-7}
    \rowcolor{gray!25} RingMo~\cite{sun2022ringmo} & Remote sensing images & Generative & Model fine-tuning & - & - & Remote sensing image analysis \\
    \cline{1-7}
    RingMo-Sense~\cite{yao2023ringmo} & Remote sensing images & Generative & Model fine-tuning & - & - & Remote sensing spatiotemporal prediction \\
    \cline{1-7}
    \rowcolor{gray!25} CSP~\cite{mai2023csp} & Remote sensing images & Contrastive & Model fine-tuning & - & - & Satellite image classification \\
    \cline{1-7}
    FourCastNet~\cite{pathak2022fourcastnet} & Grid-based meteorological data & Generative & - & - & - & Weather forecasting, tropical cyclones tracking \\
    \cline{1-7}
    \rowcolor{gray!25} Pangu-Weather~\cite{bi2023accurate} & Grid-based meteorological data & Generative & - & - & - & Weather forecasting, tropical cyclones tracking \\
    \cline{1-7}
    FengWu~\cite{chen2023fengwu} & Grid-based meteorological data & Generative & - & - & - & Weather forecasting, tropical cyclones tracking \\
    \cline{1-7}
    \rowcolor{gray!25} ClimaX~\cite{nguyen2023climax} & Grid-based meteorological data & Generative & Model fine-tuning & - & - & Weather and climate modeling \\
    \cline{1-7}
    W-MAE~\cite{man2023w} & Grid-based meteorological data & Generative & Model fine-tuning & - & - & Weather forecasting, precipitation forecasting \\
    \cline{1-7}
    \cline{1-7}
    \rowcolor{gray!25} SAMRS~\cite{wang2023samrs}, RSPrompter~\cite{chen2023rsprompter} & Remote sensing images & - & Prompt engineering & - & General to remote sensing & Remote sensing semantic segmentation \\
    Roberts et al.~\cite{roberts2023charting} & Remote sensing images & - & Prompt engineering & - & General to remote sensing & Remote sensing image analysis \\
    \cline{1-7}
    \rowcolor{gray!25} GeoSAM~\cite{sultan2023geosam} & Remote sensing images & - & Model fine-tuning & - & General to remote sensing & Mobility infrastructure segmentation \\
    \cline{1-7}
    RingMo-SAM~\cite{yan2023ringmo} & Remote sensing images & - & Model fine-tuning & - & General to remote sensing & Multi-source remote sensing segmentation \\
    \cline{1-7}
    \rowcolor{gray!25} Zhang et al.~\cite{zhang2022migratable} & Street-view images & - & Model fine-tuning & - & General to street scene sensing & Street-view image analysis \\
    \cline{1-7}
    StreetCLIP~\cite{sultan2023geosam} & Street-view images & - & Model fine-tuning & - & General to street scene sensing & Image geolocalization \\
    \midrule[0.5pt]
    
    % Trajectory-based Models
    \multicolumn{7}{c}{\textbf{Trajectory-based Models}} \\
    \cline{1-7}
    \rowcolor{gray!25} t2vec~\cite{t2vec2018} & Trajectory in road networks & Generative & Model fine-tuning & - & - & Similar trajectory search \\
    \cline{1-7}
    traj2vec~\cite{traj2vec2017} & Trajectory in road networks & Generative & Model fine-tuning & - & - & Trajectory cluster \\
    \cline{1-7}
    \rowcolor{gray!25} Trembr~\cite{Trembr2020} & Trajectory in road networks & Generative & Model fine-tuning & - & - & Similar trajectory search, travel time estimation, location prediction \\
    \cline{1-7}
    Toast~\cite{toast2021} & Trajectory in road networks & Generative & Model fine-tuning & - & - & Road classification, similar trajectory search, travel time estimation \\
    \cline{1-7}
    \rowcolor{gray!25} PIM~\cite{pim2021} & Trajectory in road networks & Contrastive & Model fine-tuning & - & - & Travel time estimation, path ranking \\
    \cline{1-7}
    STPT~\cite{stpt2023} & Trajectory in road networks & Contrastive & Model fine-tuning & - & - & Trajectory classification \\
    \cline{1-7}
    \rowcolor{gray!25} LightPath~\cite{lightpath2023} & Trajectory in road networks & Generative & Model fine-tuning & - & - & Travel time estimation, path ranking \\
    \cline{1-7}
    MMTEC~\cite{mmtec2023} & Trajectory in road networks & Maximum Entropy Coding & Prompt engineering & - & - & Similar trajectory search, travel time estimation,  location prediction. \\
    \cline{1-7}
    \rowcolor{gray!25} START~\cite{start2023} & Trajectory in road networks & Generative, contrastive & Prompt engineering & - & - & Travel time estimation, trajectory classification, similar trajectory search \\
    \cline{1-7}
    HMTRL~\cite{hmtrl2022} & Trajectory in road networks & Generative, contrastive & Model fine-tuning & - & - & Route recommendation \\
    \cline{1-7}
    \rowcolor{gray!25} Movesim~\cite{movesim2020} & Trajectory in free space & Generative, contrastive & - & - & - & Human mobility simulation \\
    \cline{1-7}
    SML~\cite{sml2021} & Trajectory in free space & Contrastive & Model fine-tuning & - & - & Location prediction, trajectory–user linking \\
    \cline{1-7}
    \rowcolor{gray!25} CTLE~\cite{ctle2021} & Trajectory in free space & Generative & - & - & - & Location prediction \\
    \cline{1-7}
    CACSR~\cite{cacsr2023} & Trajectory in free space & Contrastive & Model fine-tuning & - & - & Location prediction, trajectory user linking \\
    \cline{1-7}
    \rowcolor{gray!25} Reformd~\cite{Reformd2021} & Trajectory in free space & - & Model fine-tuning & - & - & Mobility prediction \\
    \cline{1-7}
    Axolotl~\cite{Axolotl2022} & Trajectory in free space & - & Model fine-tuning & - & - & Location recommendation \\
    \cline{1-7}
    \rowcolor{gray!25} CATUS~\cite{CATUS2023} & Trajectory in free space & Contrastive & Model fine-tuning & - & - & Location prediction \\
    \cline{1-7}
    AuxMobLCast~\cite{auxmoblcast2022} & Mobility prompt, user instructions & - & Prompt engineering & LLM for trajectory & General to human mobility & Human mobility forecasting \\
    \cline{1-7}
    \rowcolor{gray!25} LLM-Mob~\cite{llmmob2023} & Mobility prompt, user instructions & - & Prompt engineering & LLM for trajectory & General to human mobility & Location prediction \\
    \cline{1-7}
    Zhang et al.~\cite{zhang2023large} & Mobility prompt, user instructions & - & Prompt engineering & LLM for trajectory & General to human mobility & Anomalous trajectory detection \\
    \cline{1-7}
    \rowcolor{gray!25} LLM-MPE~\cite{llmmpe2023} & Mobility prompt, user instructions & - & Prompt engineering & LLM for trajectory & General to human mobility & Human mobility forecasting \\
    \cline{1-7}
    Keysan et al.~\cite{keysan2023can} & Text description of scene, user instructions & - & Prompt engineering & LLM for trajectory & General to autonomous driving & Motion planning, driving trajectory prediction \\
    \cline{1-7}
    \rowcolor{gray!25} GPT-Driver~\cite{gptdriver2023} & Text description of scene, user instructions & - & Prompt engineering & LLM for trajectory & General to autonomous driving & Motion planning, driving trajectory prediction \\
    \cline{1-7}
    LanguageMPC~\cite{languagempc2023} & Text description of scene, user instructions & - & Prompt engineering & LLM for trajectory & General to autonomous driving & Motion planning, driving trajectory prediction \\
    \midrule[0.5pt]
    
    % Time series-based Models
    \multicolumn{7}{c}{\textbf{Time series-based Models}} \\
    \cline{1-7}
    \rowcolor{gray!25} Oreshkin et al.~\cite{oreshkin2021meta} & Ordinary time series & Supervised & - & - & Electricity to traffic & Energy consumption forecasting, traffic forecasting\\
    \cline{1-7}
    Lag-Llama~\cite{rasul2023lag} & Ordinary time series & Supervised & - & - & General to traffic & Traffic forecasting\\
    \cline{1-7}
    \rowcolor{gray!25} SASA~\cite{cai2021time} & Ordinary time series & Supervised & - & - & - & Air quality regression\\
    \cline{1-7}
    TST~\cite{zerveas2021transformer} & Ordinary time series & Generative & - & - & - & Traffic regression\\
    \cline{1-7}
    \rowcolor{gray!25} SimMTM~\cite{dong2023simmtm} & Ordinary time series & Generative & - & - & Weather to traffic & Weather, energy consumption and traffic forecasting\\
    \cline{1-7}
    PatchTST~\cite{nie2022time} & Ordinary time series & Generative & - & - & Electricity to others & Weather, energy consumption and traffic forecasting\\
    \cline{1-7}
    \rowcolor{gray!25} TSMixer~\cite{ekambaram2023tsmixer} & Ordinary time series & Generative & - & - & - & Weather, energy consumption and traffic forecasting\\
    \cline{1-7}
    PT-Tuning~\cite{liu2023pt} & Ordinary time series & Generative & Prompt engineering & - & - & Weather, energy consumption and traffic forecasting\\
    \cline{1-7}
    \rowcolor{gray!25} T-Loss~\cite{franceschi2019unsupervised} & Ordinary time series & Contrastive & - & - & - & Traffic and energy consumption forecasting\\
    \cline{1-7}
    COST~\cite{woo2022cost} & Ordinary time series & Contrastive & - & - & - & Weather, energy consumption and traffic forecasting\\
    \cline{1-7}
    \rowcolor{gray!25} TS2Vec~\cite{yue2022ts2vec} & Ordinary time series & Contrastive & - & - & - & Traffic and energy consumption classification\\
    \cline{1-7}
    SimTS~\cite{zheng2023simts} & Ordinary time series & Contrastive & - & - & - & Weather and traffic forecasting\\
    \cline{1-7}
    \rowcolor{gray!25} UniTime~\cite{liu2023unitime} & Ordinary time series & Hybrid & - & - & General to urban time series & Weather, energy consumption and traffic forecasting\\
    \cline{1-7}
    ST-GSP~\cite{zhao2022st} & Spatial time series & Generative & - & - & - & Traffic forecasting\\
    \cline{1-7}
    \rowcolor{gray!25} STGCL~\cite{liu2022contrastive} & Spatial time series & Contrastive & - & - & - & Traffic forecasting\\
    \cline{1-7}
    STEP~\cite{shao2022pre} & Spatial time series & Generative & - & - & - & Traffic forecasting\\
    \cline{1-7}
    \rowcolor{gray!25} TransGTR~\cite{jin2023transferable} & Spatial time series & Hybrid & - & - & - & Traffic forecasting\\
    \cline{1-7}
    MC-STL~\cite{zhang2023mask} & Spatial time series & Hybrid & - & - & - & Traffic forecasting\\
    \cline{1-7}
    \rowcolor{gray!25} TPB~\cite{liu2023cross} & Spatial time series & Hybrid & - & - & - & Traffic forecasting\\
    \cline{1-7}
    GPT-ST~\cite{li2023gpt} & Spatial time series & Generative & - & - & - & Traffic forecasting\\
    \cline{1-7}
    \rowcolor{gray!25} PromptST~\cite{zhang2023promptst} & Spatial time series & - & Prompt tuning & - & - & Traffic and complaint forecasting\\
    \cline{1-7}
    MetePFL~\cite{chen2023prompt} & Spatial time series & - & Prompt tuning & - & - & Weather forecasting\\
    \cline{1-7}
    \rowcolor{gray!25} FedWing~\cite{chen2023spatial} & Spatial time series & - & Prompt tuning & - & - & Weather forecasting\\
    \cline{1-7}
    PromptCast~\cite{xue2023promptcast} & Ordinary time series & - & Prompt engineering & LLM for time series & Language to time series & Weather, energy consumption and human mobility forecasting\\
    \cline{1-7} 
    \rowcolor{gray!25} LLMTime~\cite{gruver2023large} & Ordinary time series & - & Prompt engineering & LLM for time series & Language to time series & Weather, energy consumption and traffic forecasting\\
    \cline{1-7} 
    GPT(6)~\cite{zhou2023one1_nips} & Ordinary time series & - & Model fine-tuning & LLM for time series & Language to time series & Weather, energy consumption and traffic forecasting\\
    \cline{1-7} 
    \rowcolor{gray!25} GPT(6)-adapter~\cite{zhou2023one2} & Ordinary time series & - & Model fine-tuning & LLM for time series & Language to time series & Weather, energy consumption and traffic forecasting\\
    \cline{1-7} 
    LLM4TS~\cite{chang2023llm4ts} & Ordinary time series & - & Model fine-tuning & LLM for time series & Language to time series & Weather, energy consumption and traffic forecasting\\
    \cline{1-7} 
    \rowcolor{gray!25} TEMPO~\cite{cao2023tempo} & Ordinary time series & - & Model fine-tuning & LLM for time series & Language to time series & Weather, energy consumption and traffic forecasting\\
    \cline{1-7} 
    GATGPT~\cite{chen2023gatgpt} & Spatial time series & - & Model fine-tuning & LLM for time series & Language to time series & Traffic forecasting, air quality imputation\\
    \cline{1-7} 
    \rowcolor{gray!25} V2S~\cite{yang2021voice2series} & Ordinary time series & - & Model Reprogramming & LLM for time series & Speech to time series & Traffic classification\\
    \cline{1-7} 
    Time-LLM~\cite{jin2023time} & Ordinary time series & - & Model reprogramming & LLM for time series & Language to time series & Traffic forecasting\\
    \cline{1-7}
    \rowcolor{gray!25} TEST~\cite{sun2023test} & Ordinary time series & - & Model reprogramming & LLM for time series & Language to time series & Traffic, energy consumption and air quality forecasting\\
    \midrule[0.5pt]

    % Multimodal Models
    \multicolumn{7}{c}{\textbf{Multimodal Models}} \\
    \cline{1-7}
    \rowcolor{gray!25} UrbanCLIP~\cite{yan2023urban} & Satellite image, textual description	& Contrastive & Model fine-tuning & LLM for image & General to urban science & Urban region profiling \\
    \cline{1-7}
    TengYun~\cite{zhao2023parallel} & Traffic-related text and image & Generative & Prompt tuning & - & - & Traffic prediction and control, transportation planning \\
    \cline{1-7}
    \rowcolor{gray!25} CityFM~\cite{balsebre2023city} & Spatial, visual, and textual geo-data & Contrastive	& -	& -	& -	& Traffic speed inference, building functionality classification\\
    \cline{1-7}
    AllSpark~\cite{shao2023allspark} & Text, image, trajectory, graph, etc.	& Contrastive &	Prompt engineering & - & - & Spatiotemporal data analysis \\
    \cline{1-7}
    \rowcolor{gray!25} TrafficGPT~\cite{zhang2023trafficgpt} & Multimodal traffic data & - & Prompt engineering & - & General to traffic management & Traffic management \\
    \cline{1-7}
    GeoGPT~\cite{zhang2023geogpt} & Multimodal geospatial data	& -	& Prompt tuning	& -	& General to geospatial & Autonomous geospatial data collection, processing, and analysis \\
    \cline{1-7}
    \rowcolor{gray!25} VELMA~\cite{schumann2023velma} & Street image, navigation instruction	& -	& Model fine-tuning	& LLM for image	& General to urban navigation & Autonomous street navigation \\
    \cline{1-7}
    UGI~\cite{xu2023urban} & Urban textual, visual, knowledge graph, human behavior data & - & Continue learning,  model fine-tuning & - & General to urban environment & Urban planning and simulation, location recommendation \\
    % \bottomrule[1pt]
\end{tabularx}
\normalsize
\twocolumn
