# Supplementary material for: Towards Urban General Intelligence: A Review and Outlook of Urban Foundation Models
Source: arXiv:2402.01749 source file (2026-03-22)
Supplement: Supplementary file 3 [file v2_appendix.tex]

\onecolumn
% \small % 或 \footnotesize 或 \scriptsize
\begin{longtable}{m{5mm}|m{3cm}m{3cm}m{2cm}m{3cm}m{4cm}}
    \caption{Summary of existing works.} \label{table:summary} \\
    \toprule
    \textbf{} & \textbf{Study} & \textbf{Data Type} & \textbf{Pre-training} & \textbf{Adaptation} & \textbf{Application} \\
    \midrule
    \endfirsthead

    \multicolumn{6}{c}{{\bfseries Table \thetable\ Summary of existing works (continued).}} \\
    \toprule
    \textbf{} & \textbf{Study} & \textbf{Data Type} & \textbf{Pre-training} & \textbf{Adaptation} & \textbf{Application} \\
    \midrule
    \endhead

    \midrule
    \multicolumn{6}{r}{{Continued on next page}} \\ 
    \endfoot

    \bottomrule
    \endlastfoot

    \multirow{10}{*}{\rotatebox{90}{\textbf{Language-based Models}}} & ERNIE-GeoL~\cite{huang2022ernie} & POI corpus, user behavior logs & Generative & Model fine-tuning & Map services \\
    \cline{2-6}
    ~ & MGeo~\cite{ding2023mgeo} & POI corpus & Generative, contrastive & Model fine-tuning & Query-POI matching \\
    \cline{2-6}
    ~ & Ji et al.~\cite{ji2023evaluating} & Geo-text, user instructions & - & Prompt engineering & Geographic information systems \\
    \cline{2-6}
    ~ & Bhandari et al.~\cite{bhandari2023large} & Geo-text, user instructions & - & Prompt engineering & Geographic information systems \\
    \cline{2-6}
    ~ & GPT4GEO~\cite{roberts2023gpt4geo} & Geo-text, user instructions & - & Prompt engineering & Geographic information systems \\
    \cline{2-6}
    ~ & Mooney et al.~\cite{mooney2023towards} & Geo-text, user instructions & - & Prompt engineering & Geographic information systems \\
    \cline{2-6}
    ~ & Mai et al.~\cite{mai2023opportunities} & Geo-text, user instructions & - & Prompt engineering & Geographic information systems \\
    \cline{2-6}
    ~ & Fu et al.~\cite{fu2023towards} & Documents, geo-text, user instructions & - & Prompt engineering & Urban science \\
    \cline{2-6}
    ~ & Aghzal et al.~\cite{aghzal2023can} & Geo-text, user instructions & - & Prompt engineering & Path planning \\
    \cline{2-6}
    ~ & GeoLLM~\cite{manvi2023geollm} & POI corpus & - & Prompt engineering & Geospatial prediction \\
    \cline{2-6}
    ~ & Zheng et al.~\cite{zheng2023chatgpt} & Traffic documents, user instructions & - & Prompt engineering & Intelligent transportation \\
    \cline{2-6}
    ~ & SpaBERT~\cite{li2022spabert}, GeoLM~\cite{li2023geolm} & Geo-text & - & Model fine-tuning & Geographic language understanding \\
    \cline{2-6}
    ~ & QUERT~\cite{xie2023quert} & User behavior logs & - & Model fine-tuning & Travel query understanding \\
    \cline{2-6}
    ~ & GEDR~\cite{mei2023improving} & POI corpus, user behavior logs & - & Model fine-tuning & Query-POI matching \\
    \cline{2-6}
    ~ & Wang et al.~\cite{wang2023optimizing} & LLM-generated instructions & - & Model fine-tuning & Urban renewal \\
    \cline{2-6}
    ~ & K2~\cite{deng2023learning} & Geo-text, geoscience instructions & - & Model fine-tuning & Geoscience tasks \\
    \midrule[0.5pt]
    
    \multirow{10}{*}{\rotatebox{90}{\textbf{Vision-based Models}}} & Urban2vec~\cite{wang2020urban2vec} & Street-view images & Contrastive & Model fine-tuning & \tabincell{c}{Demographic prediction, socioeconomic prediction} \\
    \cline{2-6}
    ~ & Li et al.~\cite{li2022predicting} & Street-view images & Contrastive & Model fine-tuning & Socioeconomic prediction \\
    \cline{2-6}
    ~ & KnowCL~\cite{liu2023knowledge} & Street-view images & Contrastive & Model fine-tuning & Socioeconomic prediction \\
    \cline{2-6}
    ~ & Wang et al.~\cite{wang2022advancing} & Remote sensing images & Generative & Model fine-tuning & \tabincell{c}{Remote sensing image analysis} \\
    \cline{2-6}
    ~ & ScaleMAE~\cite{reed2023scale} & Remote sensing images & Generative & Model fine-tuning & \tabincell{c}{Remote sensing image analysis} \\
    \cline{2-6}
    ~ & Cha et al.~\cite{cha2023billion} & Remote sensing images & Generative & Model fine-tuning & \tabincell{c}{Remote sensing image analysis} \\
    \cline{2-6}
    ~ & RingMo~\cite{sun2022ringmo} & Remote sensing images & Generative & Model fine-tuning & \tabincell{c}{Remote sensing image analysis} \\
    \cline{2-6}
    ~ & RingMo-Sense~\cite{yao2023ringmo} & Remote sensing images & Generative & Model fine-tuning & \tabincell{c}{Remote sensing spatiotemporal prediction} \\
    \cline{2-6}
    ~ & CSP~\cite{mai2023csp} & Remote sensing images & Contrastive & Model fine-tuning & \tabincell{c}{Satellite image classification} \\
    \cline{2-6}
    ~ & \tabincell{c}{FourCastNet~\cite{pathak2022fourcastnet}, Pangu-Weather~\cite{bi2023accurate}, FengWu~\cite{chen2023fengwu}} & Grid-based meteorological data & Generative & - & \tabincell{c}{Weather forecasting, tropical cyclones tracking} \\
    \cline{2-6}
    ~ & ClimaX~\cite{nguyen2023climax} & Grid-based meteorological data & Generative & Model fine-tuning & \tabincell{c}{Weather and climate modeling} \\
    \cline{2-6}
    ~ & W-MAE~\cite{man2023w} & Grid-based meteorological data & Generative & Model fine-tuning & \tabincell{c}{Weather forecasting, precipitation forecasting} \\
    \cline{2-6}
    ~ & SAMRS~\cite{wang2023samrs}, RSPrompter~\cite{chen2023rsprompter} & Remote sensing images & - & Prompt engineering & \tabincell{c}{Remote sensing semantic segmentation} \\
    \cline{2-6}
    ~ & Roberts et al.~\cite{roberts2023charting} & Remote sensing images & - & Prompt engineering & \tabincell{c}{Remote sensing image analysis} \\
    \cline{2-6}
    ~ & GeoSAM~\cite{sultan2023geosam} & Remote sensing images & - & Model fine-tuning & \tabincell{c}{Mobility infrastructure segmentation} \\
    \cline{2-6}
    ~ & RingMo-SAM~\cite{yan2023ringmo} & Remote sensing images & - & Model fine-tuning & \tabincell{c}{Multi-source remote sensing segmentation} \\
    \cline{2-6}
    ~ & Zhang et al.~\cite{zhang2022migratable} & Street-view images & - & Model fine-tuning & \tabincell{c}{Street-view image analysis} \\
    \cline{2-6}
    ~ &  StreetCLIP~\cite{sultan2023geosam} & Street-view images & - & Model fine-tuning & \tabincell{c}{Image geolocalization} \\
    
    % Trajectory-based Models
    \midrule[0.5pt]
    \multirow{10}{*}{\rotatebox{90}{\textbf{Trajectory-based Models}}} & t2vec~\cite{t2vec2018} & Trajectory in road networks & Generative & Model fine-tuning & \tabincell{c}{Similar trajectory search} \\
    \cline{2-6}
    ~ & traj2vec~\cite{traj2vec2017} & Trajectory in road networks & Generative & Model fine-tuning & \tabincell{c}{Trajectory cluster} \\
    \cline{2-6}
    ~ & Trembr~\cite{Trembr2020} & Trajectory in road networks & Generative & Model fine-tuning & \tabincell{c}{Similar trajectory search, travel time estimation, destination prediction} \\
    \cline{2-6}
    ~ & Toast~\cite{toast2021} & Trajectory in road networks & Generative & Model fine-tuning & \tabincell{c}{Road label classification, traffic inference, trajectory similarity search, travel time estimation} \\
    \cline{2-6}
    ~ & PIM~\cite{pim2021} & Trajectory in road networks & Contrastive & Model fine-tuning & \tabincell{c}{Travel time estimation, path ranking} \\
    \cline{2-6}
    ~ & STPT~\cite{stpt2023} & Trajectory in road networks & Contrastive & Model fine-tuning & \tabincell{c}{Trajectory classification, driving activity identification} \\
    \cline{2-6}
    ~ & LightPath~\cite{lightpath2023} & Trajectory in road networks & Generative & Model fine-tuning & \tabincell{c}{Travel time estimation, path ranking} \\
    \cline{2-6}
    ~ & MMTEC~\cite{mmtec2023} & Trajectory in road networks & Maximum Entropy Coding & Prompt engineering & \tabincell{c}{Similar trajectory search, travel time estimation,  destination prediction.} \\
    \cline{2-6}
    ~ & START~\cite{start2023} & Trajectory in road networks & \tabincell{c}{Generative, contrastive} & Prompt engineering & \tabincell{c}{Travel time estimation, trajectory classification, most similar trajectory search} \\
    \cline{2-6}
    ~ & HMTRL~\cite{hmtrl2022} & Trajectory in road networks & \tabincell{c}{Generative, contrastive} & Model fine-tuning & \tabincell{c}{Route recommendation} \\
    \cline{2-6}
    ~ & Movesim~\cite{movesim2020} & Trajectory in free space & \tabincell{c}{Generative, contrastive} & - & \tabincell{c}{Human mobility simulation} \\
    \cline{2-6}
    ~ & SML~\cite{sml2021} & Trajectory in free space & Contrastive & Model fine-tuning & \tabincell{c}{Location prediction, trajectory–user linking} \\
    \cline{2-6}
    ~ &  CTLE~\cite{ctle2021} & Trajectory in free space & Generative & - & \tabincell{c}{Next location prediction} \\
    \cline{2-6}
    ~ &  CACSR~\cite{cacsr2023} & Trajectory in free space & Contrastive & Model fine-tuning & \tabincell{c}{Next location prediction, trajectory user linking} \\
    \cline{2-6}
    ~ &  Reformd~\cite{Reformd2021} & Trajectory in free space & - & Model fine-tuning & \tabincell{c}{Mobility prediction} \\
    \cline{2-6}
    ~ &  Axolotl~\cite{Axolotl2022} & Trajectory in free space & - & Model fine-tuning & \tabincell{c}{Next location recommendation} \\
    \cline{2-6}
    ~ &  CATUS~\cite{CATUS2023} & Trajectory in free space & Contrastive & Model fine-tuning & \tabincell{c}{Next location prediction} \\
    \cline{2-6}
    ~ &  AuxMobLCast~\cite{auxmoblcast2022} & \tabincell{c}{Mobility prompt, user instructions} & - & Prompt engineering & \tabincell{c}{Human mobility forecasting} \\
    \cline{2-6}
    ~ &  LLM-Mob~\cite{llmmob2023} & \tabincell{c}{Mobility prompt, user instructions} & - & Prompt engineering & \tabincell{c}{Next location prediction} \\
    \cline{2-6}
    ~ &  Zhang et al.~\cite{zhang2023large} & \tabincell{c}{Mobility prompt, user instructions} & - & Prompt engineering & \tabincell{c}{Anomalous trajectory detection} \\
    \cline{2-6}
    ~ &  LLM-MPE~\cite{llmmpe2023} & \tabincell{c}{Mobility prompt, user instructions} & - & Prompt engineering & \tabincell{c}{Human mobility forecasting} \\
    \cline{2-6}
    ~ &  Keysan et al.~\cite{keysan2023can} & \tabincell{c}{Text description of scene, user instructions} & - & Prompt engineering & \tabincell{c}{Motion planning, driving trajectory prediction} \\
    \cline{2-6}
    ~ &  GPT-Driver~\cite{gptdriver2023} & \tabincell{c}{Text description of scene, user instructions} & - & Prompt engineering & \tabincell{c}{Motion planning, driving trajectory prediction} \\
    \cline{2-6}
    ~ &  LanguageMPC~\cite{languagempc2023} & \tabincell{c}{Text description of scene, user instructions} & - & Prompt engineering & \tabincell{c}{Motion planning, driving trajectory prediction} \\
    
    % Time series-based Models
    \midrule[0.5pt]
    \multirow{33}{*}{\rotatebox{90}{\textbf{Time series-based Models}}} 
    & Oreshkin et al.~\cite{oreshkin2021meta} & Ordinary time series & Supervised & - & \tabincell{c}{Energy consumption forecasting, traffic forecasting}\\
    \cline{2-6}
    ~ & Lag-Llama~\cite{rasul2023lag} & Ordinary time series & Supervised & - & Traffic forecasting\\
    \cline{2-6}
    ~ & SASA~\cite{cai2021time} & Ordinary time series & Supervised & - & Air quality regression\\
    \cline{2-6}
    ~ & TST~\cite{zerveas2021transformer} & Ordinary time series & Generative & - & Traffic regression\\
    \cline{2-6}
    ~ & SimMTM~\cite{dong2023simmtm} & Ordinary time series & Generative & - & \tabincell{c}{Weather forecasting, energy consumption forecasting, traffic forecasting}\\
    \cline{2-6}
    ~ & PatchTST~\cite{nie2022time} & Ordinary time series & Generative & - & \tabincell{c}{Weather forecasting, energy consumption forecasting, traffic forecasting}\\
    \cline{2-6}
    ~ & TSMixer~\cite{ekambaram2023tsmixer} & Ordinary time series & Generative & - & \tabincell{c}{Weather forecasting, energy consumption forecasting, traffic forecasting}\\
    \cline{2-6}
    ~ & PT-Tuning~\cite{liu2023pt} & Ordinary time series & Generative & Prompt engineering & \tabincell{c}{Weather forecasting, energy consumption forecasting, traffic forecasting}\\
    \cline{2-6}
    ~ & T-Loss~\cite{franceschi2019unsupervised} & Ordinary time series & Contrastive & - & \tabincell{c}{Traffic forecasting, energy consumption forecasting}\\
    \cline{2-6}
    ~ & COST~\cite{woo2022cost} & Ordinary time series & Contrastive & - & \tabincell{c}{Weather forecasting, energy consumption forecasting, traffic forecasting}\\
    \cline{2-6}
    ~ & TS2Vec~\cite{yue2022ts2vec} & Ordinary time series & Contrastive & - & \tabincell{c}{Traffic classification, energy consumption classification}\\
    \cline{2-6}
    ~ & SimTS~\cite{zheng2023simts} & Ordinary time series & Contrastive & - & \tabincell{c}{Weather forecasting, traffic forecasting}\\
    \cline{2-6}
    ~ & UniTime~\cite{liu2023unitime} & Ordinary time series & Hybrid & - & \tabincell{c}{Weather forecasting, energy consumption forecasting, traffic forecasting}\\
    \cline{2-6}
    ~ & ST-GSP~\cite{zhao2022st} & Spatial time series & Generative & - & Traffic forecasting\\
    \cline{2-6}
    ~ & STGCL~\cite{liu2022contrastive} & Spatial time series & Contrastive & - & Traffic forecasting\\
    \cline{2-6}
    ~ & STEP~\cite{shao2022pre} & Spatial time series & Generative & - & Traffic forecasting\\
    \cline{2-6}
    ~ & TransGTR~\cite{jin2023transferable} & Spatial time series & Hybrid & - & Traffic forecasting\\
    \cline{2-6}
    ~ & MC-STL~\cite{zhang2023mask} & Spatial time series & Hybrid & - & Traffic forecasting\\
    \cline{2-6}
    ~ & TPB~\cite{liu2023cross} & Spatial time series & Hybrid & - & Traffic forecasting\\
    \cline{2-6}
    ~ & GPT-ST~\cite{li2023gpt} & Spatial time series & Generative & - & Traffic forecasting\\
    \cline{2-6}
    ~ & PromptST~\cite{zhang2023promptst} & Spatial time series & - & Prompt engineering & \tabincell{c}{Traffic forecasting, complaint forecasting}\\
    \cline{2-6}
    ~ & MetePFL~\cite{chen2023prompt} & Spatial time series & - & Prompt engineering & Weather forecasting\\
    \cline{2-6}
    ~ & FedWing~\cite{chen2023spatial} & Spatial time series & - & Prompt engineering & Weather forecasting\\
    \cline{2-6}
    ~ & PromptCast~\cite{xue2023promptcast} & Ordinary time series & - & Prompt engineering & \tabincell{c}{Weather forecasting, energy consumption forecasting, human mobility forecasting}\\
    \cline{2-6} 
    ~ & LLMTime~\cite{gruver2023large} & Ordinary time series & - & Prompt engineering & \tabincell{c}{Weather forecasting, energy consumption forecasting, traffic forecasting}\\
    \cline{2-6} 
    ~ & GPT(6)~\cite{zhou2023one1_nips} & Ordinary time series & - & Model fine-tuning & \tabincell{c}{Weather forecasting, energy consumption forecasting, traffic forecasting}\\
    \cline{2-6} 
    ~ & GPT(6)-adapter~\cite{zhou2023one2} & Ordinary time series & - & Model fine-tuning & \tabincell{c}{Weather forecasting, energy consumption forecasting, traffic forecasting}\\
    \cline{2-6} 
    ~ & LLM4TS~\cite{chang2023llm4ts} & Ordinary time series & - & Model fine-tuning & \tabincell{c}{Weather forecasting, energy consumption forecasting, traffic forecasting}\\
    \cline{2-6} 
    ~ & TEMPO~\cite{cao2023tempo} & Ordinary time series & - & Model fine-tuning & \tabincell{c}{Weather forecasting, energy consumption forecasting, traffic forecasting}\\
    \cline{2-6} 
    ~ & GATGPT~\cite{chen2023gatgpt} & Spatial time series & - & Model fine-tuning & \tabincell{c}{Traffic forecasting, air quality imputation}\\
    \cline{2-6} 
    ~ & V2S~\cite{yang2021voice2series} & Ordinary time series & - & Model Reprogramming & Traffic classification\\
    \cline{2-6} 
    ~ & Time-LLM~\cite{jin2023time} & Ordinary time series & - & Model reprogramming & Traffic forecasting\\
    \cline{2-6}
    ~ & TEST~\cite{sun2023test} & Ordinary time series & - & Model reprogramming & \tabincell{c}{Traffic forecasting, energy consumption forecasting, air quality forecasting}\\
    
    \midrule[0.5pt]
    \multirow{14}{*}{\rotatebox{90}{\textbf{Multimodal Models}}} &  UrbanCLIP~\cite{yan2023urban} & Satellite image, textual description	& Contrastive & Model fine-tuning & Urban region profiling \\
    \cline{2-6}
    ~ & TengYun~\cite{zhao2023parallel} & Traffic-related text and image & Generative & Prompt tuning & \tabincell{c}{Traffic prediction and control, transportation planning} \\
    \cline{2-6}
    ~ & CityFM~\cite{balsebre2023city} & Spatial, visual, and textual geo-data & Contrastive	& -	& \tabincell{c}{Traffic speed inference, building functionality classification}\\
    \cline{2-6}
    ~ & AllSpark~\cite{shao2023allspark} & Text, image, trajectory, graph, etc.	& Contrastive &	Prompt engineering & Spatiotemporal data analysis \\
    \cline{2-6}
    ~ & TrafficGPT~\cite{zhang2023trafficgpt} & Multimodal traffic data & - & Prompt engineering & Traffic management \\
    \cline{2-6}
    ~ & GeoGPT~\cite{zhang2023geogpt} & Multimodal geospatial data	& -	& Prompt tuning	& \tabincell{c}{Autonomous geospatial data collection, processing, and analysis} \\
    \cline{2-6}
    ~ & VELMA~\cite{schumann2023velma} & Street image, navigation instruction	& -	& Model fine-tuning	& Autonomous street navigation \\
    \cline{2-6}
    ~ & UGI~\cite{xu2023urban} & \tabincell{c}{Urban textual, visual, knowledge graph, human behavior data} & - & \tabincell{c}{Continue learning, model fine-tuning} & \tabincell{c}{Urban planning and simulation, location recommendation} \\
    % \bottomrule[1pt]
\end{longtable}
\normalsize
\twocolumn
