# Supplementary material for: Towards Urban General Intelligence: A Review and Outlook of Urban Foundation Models
Source: arXiv:2402.01749 source file (2026-03-22)
Supplement: Supplementary file 4 [file v3_appendix.tex]

\appendix[Summary of Existing Works
]

\onecolumn
% \small
\footnotesize
% \rowcolors{3}{gray!25}{white}
\begin{longtable}{ 
    >{\centering\arraybackslash}m{2.5cm}
    >{\centering\arraybackslash}m{2cm}
    >{\centering\arraybackslash}m{2cm}
    >{\centering\arraybackslash}m{2cm}
    >{\centering\arraybackslash}m{2cm}
    >{\centering\arraybackslash}m{2cm}
    >{\centering\arraybackslash}m{2cm}
    }
    \caption{Summary of existing works.} \label{table:summary} \\
    \toprule
    % \rowcolor{gray!50}
    \textbf{Study} & \textbf{Data Type} & \textbf{Pre-training} & \textbf{Adaptation} & \textbf{Cross-modal transfer} & \textbf{Cross-domain transfer} & \textbf{Application} \\
    \midrule
    \endfirsthead

    \multicolumn{7}{c}{{\bfseries Table \thetable\ Summary of existing works (continued).}} \\
    \toprule
    % \rowcolor{gray!50}
    \textbf{Study} & \textbf{Data Type} & \textbf{Pre-training} & \textbf{Adaptation} & \textbf{Cross-modal transfer} & \textbf{Cross-domain transfer} & \textbf{Application} \\
    \midrule
    \endhead

    \midrule
    \multicolumn{7}{r}{{Continued on next page}} \\ 
    \endfoot

    \bottomrule
    \endlastfoot

    \multicolumn{7}{c}{\textbf{Language-based Models}} \\
    \hline
    ERNIE-GeoL~\cite{huang2022ernie} & POI corpus, user behavior logs & Generative & Model fine-tuning & - & - & Map services \\
    \cline{1-7}
    \rowcolor{gray!25} MGeo~\cite{ding2023mgeo} & POI corpus & Generative, contrastive & Model fine-tuning & - & - & Query-POI matching \\
    \cline{1-7}
    Ji et al.~\cite{ji2023evaluating} & Geo-text, user instructions & - & Prompt engineering & - & General to geospatial & Geographic information systems \\
    \cline{1-7}
    \rowcolor{gray!25} Bhandari et al.~\cite{bhandari2023large} & Geo-text, user instructions & - & Prompt engineering & - & General to geospatial & Geographic information systems \\
    \cline{1-7}
    GPT4GEO~\cite{roberts2023gpt4geo} & Geo-text, user instructions & - & Prompt engineering & - & General to geospatial & Geographic information systems \\
    \cline{1-7}
    \rowcolor{gray!25} Mooney et al.~\cite{mooney2023towards} & Geo-text, user instructions & - & Prompt engineering & - & General to geospatial & Geographic information systems \\
    \cline{1-7}
    Mai et al.~\cite{mai2023opportunities} & Geo-text, user instructions & - & Prompt engineering & - & General to geospatial & Geographic information systems \\
    \cline{1-7}
    \rowcolor{gray!25} Fu et al.~\cite{fu2023towards} & Documents, geo-text, user instructions & - & Prompt engineering & - & General to urban science & Urban science \\
    \cline{1-7}
    Aghzal et al.~\cite{aghzal2023can} & Geo-text, user instructions & - & Prompt engineering & - & General to path planning & Path planning \\
    \cline{1-7}
    \rowcolor{gray!25} GeoLLM~\cite{manvi2023geollm} & POI corpus & - & Prompt engineering & - & General to geospatial & Geospatial prediction \\
    \cline{1-7}
    Zheng et al.~\cite{zheng2023chatgpt} & Traffic documents, user instructions & - & Prompt engineering & - & General to transportation & Intelligent transportation \\
    \cline{1-7}
    \rowcolor{gray!25} SpaBERT~\cite{li2022spabert}, GeoLM~\cite{li2023geolm} & Geo-text & - & Model fine-tuning & - & General to geospatial & Geographic language understanding \\
    \cline{1-7}
    QUERT~\cite{xie2023quert} & User behavior logs & - & Model fine-tuning & - & General to travel domain search & Travel query understanding \\
    \cline{1-7}
    \rowcolor{gray!25} GEDR~\cite{mei2023improving} & POI corpus, user behavior logs & - & Model fine-tuning & - & General to POI search & Query-POI matching \\
    \cline{1-7}
    Wang et al.~\cite{wang2023optimizing} & LLM-generated instructions & - & Model fine-tuning & - & General to urban renewal & Urban renewal \\
    \cline{1-7}
    \rowcolor{gray!25} K2~\cite{deng2023learning} & Geo-text, geoscience instructions & - & Model fine-tuning & - & General to geoscience & Geoscience tasks \\
    \midrule[0.5pt]
    
    % Vision-based Models
    \multicolumn{7}{c}{\textbf{Vision-based Models}} \\
    \cline{1-7}
    Urban2vec~\cite{wang2020urban2vec} & Street-view images & Contrastive & Model fine-tuning & - & - & \tabincell{c}{Demographic prediction, socioeconomic prediction} \\
    \cline{1-7}
    \rowcolor{gray!25} Li et al.~\cite{li2022predicting} & Street-view images & Contrastive & Model fine-tuning & - & - & Socioeconomic prediction \\
    \cline{1-7}
    KnowCL~\cite{liu2023knowledge} & Street-view images & Contrastive & Model fine-tuning & - & - & Socioeconomic prediction \\
    \cline{1-7}
    \rowcolor{gray!25} Wang et al.~\cite{wang2022advancing} & Remote sensing images & Generative & Model fine-tuning & - & - & \tabincell{c}{Remote sensing image analysis} \\
    \cline{1-7}
    ScaleMAE~\cite{reed2023scale} & Remote sensing images & Generative & Model fine-tuning & - & - & \tabincell{c}{Remote sensing image analysis} \\
    \cline{1-7}
    \rowcolor{gray!25} Cha et al.~\cite{cha2023billion} & Remote sensing images & Generative & Model fine-tuning & - & - & \tabincell{c}{Remote sensing image analysis} \\
    \cline{1-7}
    RingMo~\cite{sun2022ringmo} & Remote sensing images & Generative & Model fine-tuning & - & - & \tabincell{c}{Remote sensing image analysis} \\
    \cline{1-7}
    \rowcolor{gray!25} RingMo-Sense~\cite{yao2023ringmo} & Remote sensing images & Generative & Model fine-tuning & - & - & \tabincell{c}{Remote sensing spatiotemporal prediction} \\
    \cline{1-7}
    CSP~\cite{mai2023csp} & Remote sensing images & Contrastive & Model fine-tuning & - & - & \tabincell{c}{Satellite image classification} \\
    \cline{1-7}
    \rowcolor{gray!25} \tabincell{c}{FourCastNet~\cite{pathak2022fourcastnet}, Pangu-Weather~\cite{bi2023accurate}, FengWu~\cite{chen2023fengwu}} & Grid-based meteorological data & Generative & - & - & - & \tabincell{c}{Weather forecasting, tropical cyclones tracking} \\
    \cline{1-7}
    ClimaX~\cite{nguyen2023climax} & Grid-based meteorological data & Generative & Model fine-tuning & - & - & \tabincell{c}{Weather and climate modeling} \\
    \cline{1-7}
    \rowcolor{gray!25} W-MAE~\cite{man2023w} & Grid-based meteorological data & Generative & Model fine-tuning & - & - & \tabincell{c}{Weather forecasting, precipitation forecasting} \\
    \cline{1-7}
    SAMRS~\cite{wang2023samrs}, RSPrompter~\cite{chen2023rsprompter} & Remote sensing images & - & Prompt engineering & - & General to remote sensing & \tabincell{c}{Remote sensing semantic segmentation} \\
    \cline{1-7}
    \rowcolor{gray!25} Roberts et al.~\cite{roberts2023charting} & Remote sensing images & - & Prompt engineering & - & General to remote sensing & \tabincell{c}{Remote sensing image analysis} \\
    \cline{1-7}
    GeoSAM~\cite{sultan2023geosam} & Remote sensing images & - & Model fine-tuning & - & General to remote sensing & \tabincell{c}{Mobility infrastructure segmentation} \\
    \cline{1-7}
    \rowcolor{gray!25} RingMo-SAM~\cite{yan2023ringmo} & Remote sensing images & - & Model fine-tuning & - & General to remote sensing & \tabincell{c}{Multi-source remote sensing segmentation} \\
    \cline{1-7}
    Zhang et al.~\cite{zhang2022migratable} & Street-view images & - & Model fine-tuning & - & General to street scene sensing & \tabincell{c}{Street-view image analysis} \\
    \cline{1-7}
    \rowcolor{gray!25} StreetCLIP~\cite{sultan2023geosam} & Street-view images & - & Model fine-tuning & - & General to street scene sensing & \tabincell{c}{Image geolocalization} \\
    
\end{longtable}
\normalsize
\twocolumn
